# Supplementary material for: Subpopulation Data Poisoning Attacks
Source: arXiv:2006.14026 source file (2021-05-12)
Supplement: Supplementary file 1 [file appendix_models.tex]

\section{Experiment Details}
\label{app:details}
Here we will provide a brief overview of the multiple models used in the experimental phase and the hyper-parameters used in training them.

\begin{itemize}

 \item For the CIFAR-10 dataset, we use \scifar\ and \lcifar. \scifar\ is a small convolutional neural network, consisting of a convolutional layer, three blocks consisting of 2 convolutional layers and an average pooling layer each, and a final convolution and reduce mean operation. This is trained with SGD using a learning rate of  and a weight decay of 0.02, following . \lcifar\ trains a VGG-16 model pretrained on ImageNet, fine tuning all layers for 12 epochs with Adam with a learning rate of 0.001.
 
 \item For UTKFace, we use \sutk\ and \lutk. \sutk only trains the last layer of a VGG-16 model pretrained on ImageNet, while \lutk\ trains all layers. For both, we train for 12 epochs with Adam w,using a learning rate of 0.001 for \sutk\ and 0.0001 for \lutk. For both, we use $\ell_2$ regularization of 0.01 on the classification layer.
   
\item For the IMDB review dataset, we use \sbert\ and \lbert. These models use the same architecture and implementation from the Huggingface Transformers library \cite{Wolf2019HuggingFacesTS}.
    They are both based on a pre-trained \verb|bert-base-uncased| instance, with 12 transformer blocks, and one linear layer for classification.
    The main difference between the two models is that for \lbert\, the entire model is fine-tuned over the IMDB training set, while with \sbert\ we freeze all the layers of the model except for the last transformer block and the classifier before fine-tuning. Both models are then fine-tuned on vectors of 256 tokens, for 4 epochs, with a learning rate of $10^{-5}$ and mini batch size of 8.

    \item For UCI Adult, we use a neural network with one hidden layer of 10 ReLU units, trained for a maximum of 3000 iterations using scikit-learn default settings for all other parameters. We drop the 'education', 'native-country', and 'fnlwgt' columns due to significant correlation with other columns, and one-hot encode categorical columns.

\end{itemize}
